# Supplementary material for: Exploring Ground and Excited States via Single Reference Coupled-Cluster Theory and Algebraic Geometry
Source: arXiv:2405.12238 source file (2024-09-10)
Supplement: Supplementary file 1 [file supporting_information.pdf]

# Supporting Information:

## Exploring Ground and Excited States via Single Reference Coupled-Cluster Theory and Algebraic Geometry

Svala Sverrisdóttir† and Fabian M. Faulstich*,‡

†*Department of Mathematics, The University of California, Berkeley, CA 94720, USA*

‡*Department of Mathematics, Rensselaer Polytechnic Institute, Troy, NY 12180, USA*

E-mail: faulsf@rpi.edu

# Dissociating systems of hydrogen

We begin by reporting the full energy spectrum of the Hamiltonian describing $(H_2)_2$ in $D_{2h}$ symmetry together with all real-valued CCD energies, see Figure S1a. Given the large number of solutions, we minimize over the difference between spectral values of the Hamiltonian and the found CCD energies. This provides further insight into energies that are well approximated by CCD, see Figure S1b.

Similarly, we proceed for $(H_2)_2$ in $D_{\infty h}$ symmetry. We reporting the full energy spectrum of the Hamiltonian describing $(H_2)_2$ in $D_{\infty h}$ symmetry together with all real-valued CCD energies, see Figure S2a Given the large number of solutions, we minimize over the difference between spectral values of the Hamiltonian and the found CCD energies. This provides further insight into energies that are well approximated by CCD, see Figure S2b.

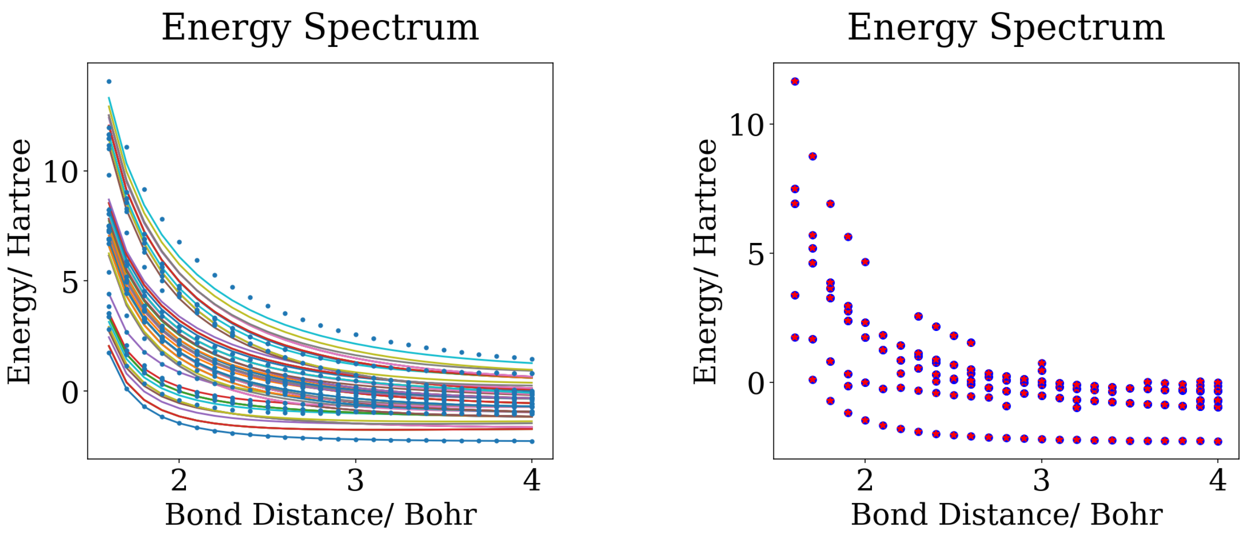


(a) (b)

Figure S1: (a) The solid lines describe the FCI spectrum. The dots correspond to real-valued CCD energies (b) Real-valued CCD energies that are close in energy to FCI energy values. The blue dots correspond to FCI energies, and the red stars correspond to CCD energies.

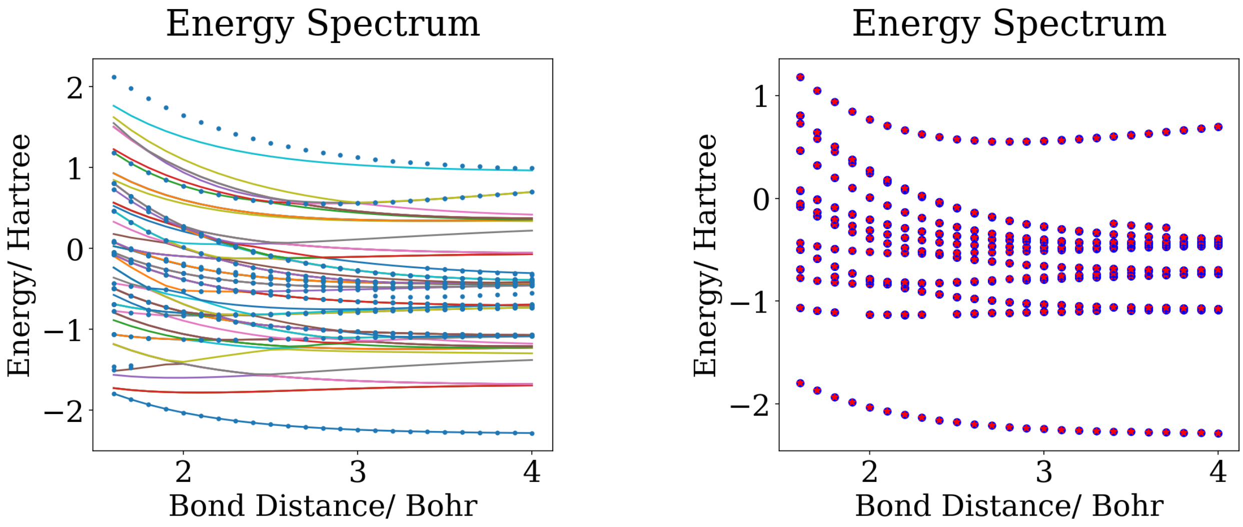


(a) (b)

Figure S2: (a) The solid lines describe the FCI spectrum. The dots correspond to real-valued CCD energies (b) Real-valued CCD energies that are close in energy to FCI energy values. The blue dots correspond to FCI energies, and the red stars correspond to CCD energies.

# $H_4$ disturbed on a circle

Similarly, we proceed for $H_4$ disturbed on a circle. We report the full energy spectrum of the Hamiltonian describing $H_4$ disturbed on a circle together with all real-valued CCD energies,

see Figure S3a. Given the large number of solutions, we minimize over the difference between spectral values of the Hamiltonian and the found CCD energies. This provides further insight into energies that are well approximated by CCD, see Figure S3b.

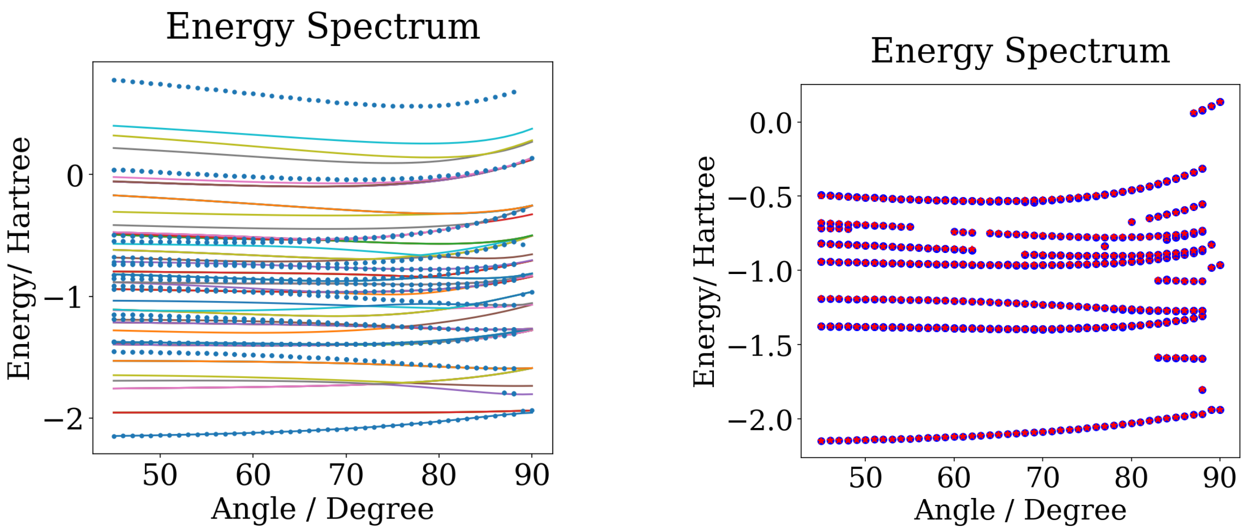


(a) (b)

Figure S3: (a) The solid lines describe the FCI spectrum. The dots correspond to real-valued CCD energies (b) Real-valued CCD energies that are close in energy to FCI energy values. The blue dots correspond to FCI energies, and the red stars correspond to CCD energies.

# Lithium hydride

We report the full energy spectrum of the Hamiltonian describing LiH together with all real-valued CCD energies, see Figure S4a Given the large number of solutions, we minimize over the difference between spectral values of the Hamiltonian and the found CCD energies. This provides further insight into energies that are well approximated by CCD, see Figure S2b.

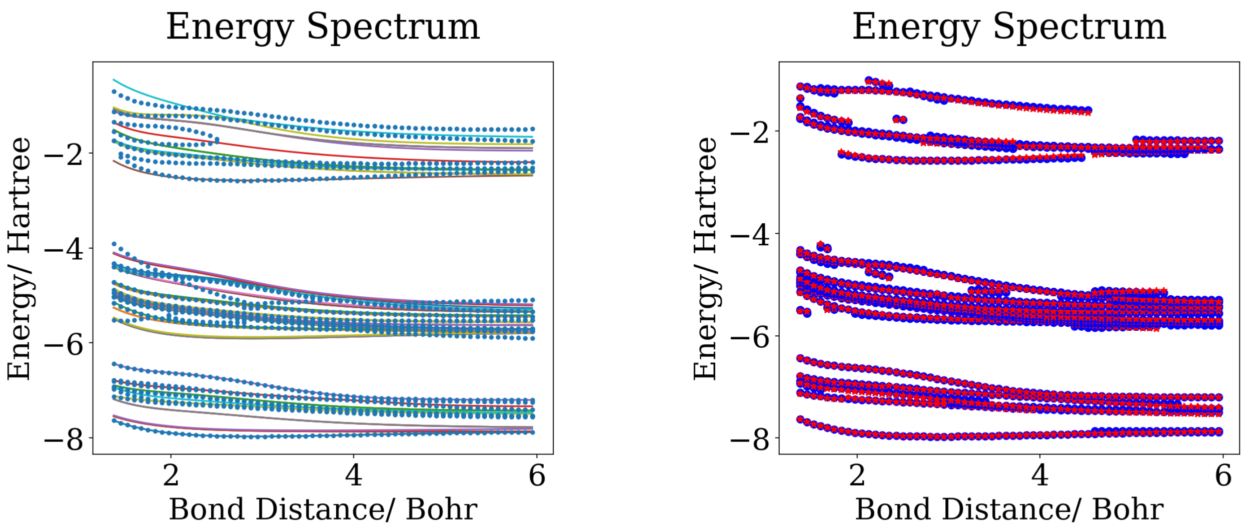


(a)

(b)

Figure S4: (a) The solid lines describe the FCI spectrum. The dots correspond to real-valued CCD energies (b) Real-valued CCD energies that are close in energy to FCI energy values. The blue dots correspond to FCI energies, and the red stars correspond to CCD energies.
